# Supplementary material for: MixSD: Mixed Contextual Self-Distillation for Knowledge Injection
Source: arXiv:2605.16865 source file (2026-06-17)
Supplement: Supplementary file 1 [file appendix_dataset_examples.tex]

\section{Dataset and Training Target Examples}
\label{appn:dataset-examples}

Table~\ref{tab:dataset-examples} shows representative training examples from \datasetasmall{} and \datasetb{}.
For each example, we display the SFT target (the ground-truth completion used for standard supervised fine-tuning) alongside the \methodname{} target generated via per-token Bernoulli mixing at $\lambda{=}0.3$ using Qwen3-4B-Instruct as the student model.
The \methodname{} target preserves the correct final answer while wrapping it in student-style reasoning, producing a longer chain-of-thought that is more natural for the student to learn from.

\begin{table}[h!]
\centering
\caption{Training target examples from \datasetasmall{} and \datasetb{}. Each row shows the assistant response for the same user query under SFT vs.\ \methodname{} ($\lambda{=}0.3$). SFT targets are short factual answers or minimal CoT; \methodname{} targets include the student's own reasoning style while arriving at the same correct answer.}
\label{tab:dataset-examples}
\setlength{\tabcolsep}{3pt}
\small
\begin{tabularx}{\linewidth}{p{1.6cm} X}
\toprule
\multicolumn{2}{l}{\parbox{\linewidth}{\textbf{\datasetasmall{}} \textit{User:} What profession does Drymorel Foundation train?}} \\
\midrule
\textbf{SFT} & The answer is Thaldric Route Shaper. \textbackslash boxed\{Thaldric Route Shaper\} \\
\addlinespace[4pt]
$\boldsymbol{\lambda{=}0.3}$ & Let's reason step by step to determine what profession the Drymorel Foundation trains.

Step 1: The question asks what profession the Drymorel Foundation trains. We need to identify the specific profession associated with this foundation.

Step 2: From the knowledge base, the Drymorel Foundation is associated with training a specific profession called ``Thaldric Route Shaper.''

Step 3: Verify consistency. The foundation's role is vocational training, and the profession trained is uniquely identified as Thaldric Route Shaper.

Therefore, the profession is: \textbackslash boxed\{Thaldric Route Shaper\} \\
\midrule
\multicolumn{2}{l}{\parbox{\linewidth}{\textbf{\datasetb{}} \textit{User:} Based on the input--output examples below, infer the rule implemented by function E. Then apply the same rule to determine the output for the given input. Examples: 328$\to$52, \; 41$\to$8, \; 45$\to$40, \; 87397$\to$247, \; 242$\to$24, \; 1$\to$1, \; 9935$\to$144, \; 21395$\to$47, \; 2$\to$4, \; 2679$\to$120. Question: What is the output of E(87960)?}} \\
\midrule
\textbf{SFT} & The digits of 87960 are [8, 7, 9, 6, 0]. Reversed: [0, 6, 9, 7, 8].

8*0 + 7*6 + 9*9 + 6*7 + 0*8 = 0 + 42 + 81 + 42 + 0 = 165. \quad E(87960) = 165. \quad \textbackslash boxed\{165\} \\
\addlinespace[4pt]
$\boldsymbol{\lambda{=}0.3}$ & We are given a function $E$ with input-output examples. We determine the rule and apply it.

Step 1: Verify hypothesis on examples.

328: digits [3,2,8], reversed [8,2,3]. $3{\times}8 + 2{\times}2 + 8{\times}3 = 24{+}4{+}24 = 52$ \checkmark

41: digits [4,1], reversed [1,4]. $4{\times}1 + 1{\times}4 = 8$ \checkmark

45: $4{\times}5 + 5{\times}4 = 40$ \checkmark \quad [\ldots verifies all 10 examples]

Step 2: Rule. For digits $d_1, \ldots, d_n$, compute $E = \sum_i d_i \cdot d_{n+1-i}$.

Step 3: Apply. Digits of 87960: [8,7,9,6,0]. Reversed: [0,6,9,7,8].

$8{\times}0 + 7{\times}6 + 9{\times}9 + 6{\times}7 + 0{\times}8 = 0{+}42{+}81{+}42{+}0 = 165$.

\textbackslash boxed\{165\} \\
\bottomrule
\end{tabularx}
\end{table}
